# Supplementary material for: Excitonic coupling dominates the homogeneous photoluminescence excitation linewidth in semicrystalline polymeric semiconductors
Source: arXiv:1702.03378 source file (2017-04-24)
Supplement: Supplementary file 1 [file Gregoire_resubmitted240417_Suppl.pdf]

# Supplemental Material: Excitonic coupling dominates the homogeneous photoluminescence excitation linewidth in semicrystalline polymeric semiconductors

Pascal Grégoire,[1] Eleonora Vella,[1] Matthew Dyson,[2,3]
Claudia M. Bazán,[1] Richard Leonelli,[1] Natalie Stingelin,[3,4]
Paul N. Stavrinou,[5] Eric R. Bittner,[6] and Carlos Silva[1,2,*]

[1]*Département de physique & Regroupement québécois sur les matériaux de pointe, Université de Montréal, C.P. 6128, Succursale centre-ville, Montréal H3C 3J7, Canada*

[2]*Department of Physics, Imperial College London, South Kensington Campus, London SW7 2AZ, United Kingdom*

[3]*Department of Materials, Imperial College London, South Kensington Campus, London SW7 2AZ, United Kingdom*

[4]*School of Materials Science and Engineering and School of Chemical and Biochemical Engineering, Georgia Institute of Technology, Atlanta, Georgia 30332-0245, USA*

[5]*Department of Engineering Science, University of Oxford, Parks Road, Oxford, OX1 3PJ, United Kingdom*

[6]*Departments of Chemistry and Physics, University of Houston, Houston, Texas 77204-5003, USA*

(Dated: April 24, 2017)

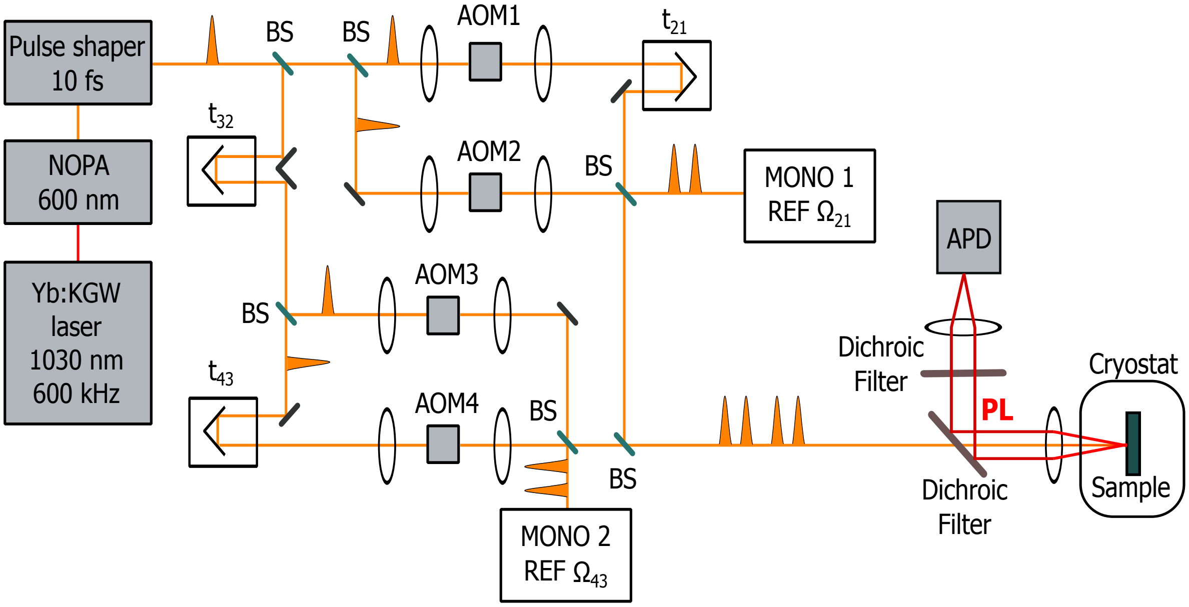


FIG. S1. Scheme for the 2D-PLE measurements. NOPA: noncollinear optical parametric amplifier; BS: Beam splitter 50/50; AOM: acousto-optic modulator; MONO: monochromator; APD: avalanche photodiode.

## SAMPLE PREPARATION

Poly(3-hexylthiophene-2,5-diyl) (P3HT), synthesised by J. de Mello and J. Bannock at Imperial College London, with weight-averaged molecular weight ($M_w$) of 113 kg mol$^{-1}$, dispersity (Đ) of 1.5, and 99% regioregularity was cast from a chloroform solution with a concentration of 10 mg mL$^{-1}$ polymer content. This was magnetically stirred at 50°C for 3 hours to ensure complete dissolution and homogeneity, before wire-bar coating (K 101 Control Coater, Printcoat Instruments) 20 $\mu$L of solution at 4 cm$^{-1}$ onto a 12-mm by 12-mm fused silica substrate (UQG Optics) at room temperature (23°C), with solvent allowed to evaporate freely.

## 2D-PLE SETUP

The 2D-PLE setup, shown in Fig. S1, is based on the phase-modulation technique introduced by Marcus and coworkers [1]. A four-pulse sequence is generated by two Mach-Zehnder intermerometers (MZI) nested in an outer MZI. This pulse sequence is derived from a noncollinear optical parametric amplifier (Light Conversion Orpheus-N-3H, 600 nm, 80 nm band-

with), pumped by the output of a regenerative amplifier (Light Conversion Pharos, 600 kHz, 1030 nm, 220 fs). An adaptive $4f$ pulse shaper (BioPhotonics Solutions FemtoJock-P) precompresses the pulse to reach the transform limit at the sample position (∼12 fs). A set of 50/50 beam splitters is used to split the pulse in four and recombine them in a collinear geometry while three optical delay lines allow to control the inter-pulse delays $t_{21}$, $t_{32}$ and $t_{43}$. In order to use the phase-modulation scheme, an acousto-optic Bragg cell is introduced in each of the four MZI arms. The first-order diffraction out of each acousto-optic cell produces a phase-modulated pulse at chosen frequency $\Omega_i$ ($i = 1, 2, 3, 4$) close to 200 MHz. When the pulse sequence is incident on the sample, the first pulse pair (pulses 1 and 2, denoted as the 'pump' pulses) produces a population signal oscillating with frequency $\Omega_{21} = \Omega_2 - \Omega_1$ while the second pulse pair (pulses 3 and 4, denoted as the 'probe' pulses) gives a signal with frequency $\Omega_{43} = \Omega_4 - \Omega_3$. The exact values $\Omega_i$ are chosen such that $\Omega_{21}$ and $\Omega_{43}$ are in the kHz range. A lock-in amplifier (Zurich Instruments HF2LI equipped with multi-frequency and AM/FM modulation modules) is then used to isolate a fourth-order contribution to the signal. The so called *rephasing* and *nonrephasing* spectra are respectively extracted at modulation frequency $\Omega_{21} - \Omega_{43}$ and $\Omega_{21} + \Omega_{43}$. In addition to those nonlinear signals, the linear excitation signal at modulation frequency $\Omega_{21}$ and $\Omega_{43}$ are also acquired simultaneously. Two monochromators equipped with avalanche photodiodes (APD) allow to construct optically the reference waveforms necessary to the lock-in for phase-sensitive detection, while amplitude modulation is used to obtain the sum and difference frequency waveforms (sideband frequencies).

The spectrally-integrated steady state photoluminescence (PL) is used as the action (excitation) signal in the experiment. The sample is maintained at 8 K in a cold-finger cryostation (Attocube) and the PL is collected in reflection geometry. We isolate the PL from the excitation laser with a set of dichroic filters, then an APD (Hamamatsu C12703-01) detects the action signal and feeds it to the lock-in amplifier. 2D coherence decay functions are obtained by measuring the demodulated PL while scanning the delays $t_{21}$ and $t_{43}$ (coherence times) keeping $t_{32}$ fixed (population time). A Fourier transformation on axes $t_{21}$ and $t_{43}$ provides the 2D spectra for a given population time.

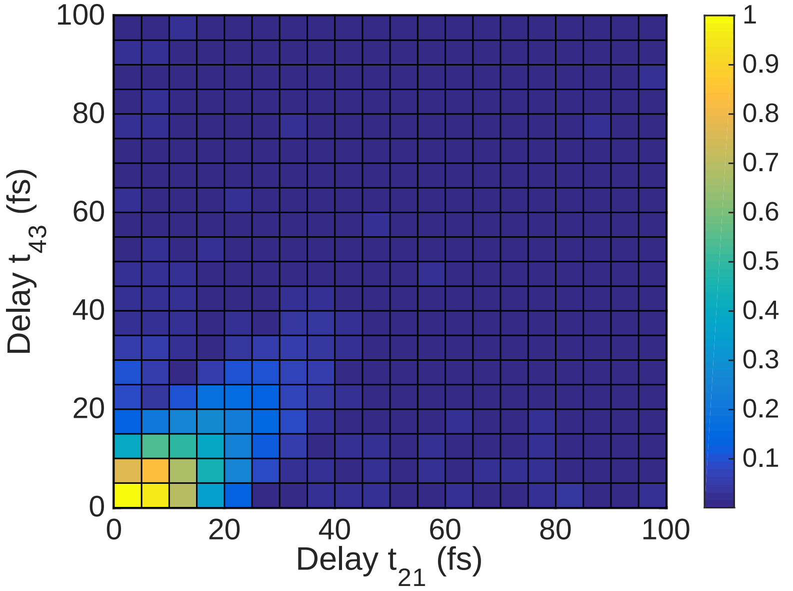


FIG. S2. Norm of the normalized 2D rephasing spectrum in the time domain. The diagonal feature shows the homogeneous dephasing time. It reaches the background noise level at $\sim 50\,fs$, which justifies the use of numerical zero padding after 100 fs.

## 2D COHERENCE DECAY FUNCTION

Figure S2 shows the raw data in the time domain for the 2D rephasing spectrum (photon echo spectrum). The elongated feature on the diagonal is characteristic of a system with homogeneous broadening smaller than the inhomogeneous distribution [2]. The signal reaches the level of the noise at $\sim$ 50 fs. We can then assume that the signal is negligible after 100 fs and numerically pad it with zeros to further increase the range on the time axes. The spectral resolution of this time-domain measurement is, in principle, limited by the measurement range in $t_{21}$ and $t_{43}$, so zero-padding has the effect of increasing the resolution to $\sim$ 20 meV and smoothing the data in the frequency domain [3].

## COMPLETE TWO-DIMENSIONAL RESPONSE

The modulus, the real part, and the imaginary part of the low temperature 2D spectra are shown in Fig. S3.

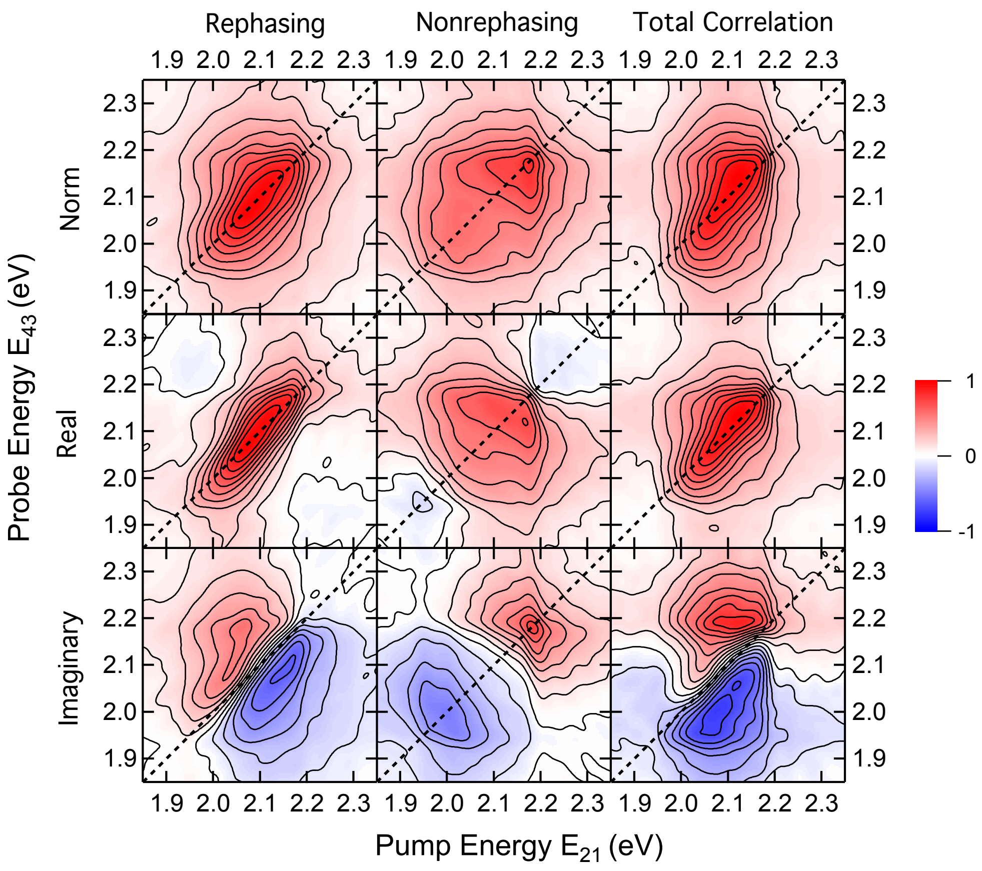


FIG. S3. Modulus, real and imaginairy parts of 2D spectra for 8 K P3HT film with $T_{32} = 50\,\text{fs}$, measured at 8 K.

## SPECTRAL LINESHAPE EVOLUTION OVER POPULATION TIME

Figure S4 displays the photon echo spectrum for population times $t_{32} = 0\,\text{fs}$, 50 fs and 1 ps. Apart from an intensity decrease, the three spectra are similar; the lineshape does not evolve significantly with $t_{32}$. Since the antidiagonal width for those three delays are essentially identical, we chose to restrict the discussion to $t_{32} = 50\,\text{fs}$, to avoid any possible pulse overlap effect at $t_{32} = 0\,\text{fs}$. This absence of evolution is consistent with a strict separation of timescales, were homogeneous dephasing is much faster than any inhomogeneous process [3].

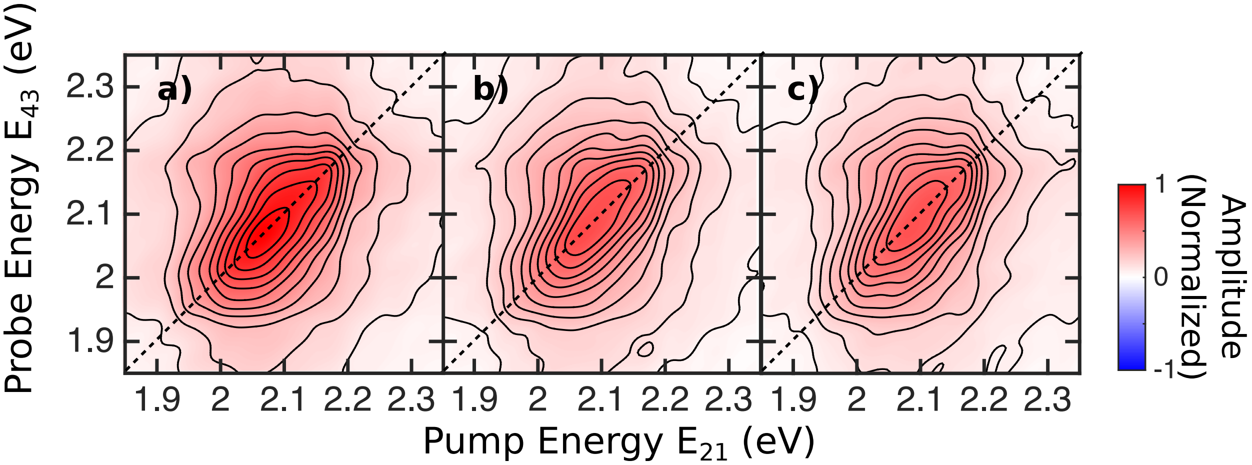


FIG. S4. Photon echo spectrum for a population waiting time of a) 0 fs, b) 50 fs and c) 1 ps. The lineshape does not significantly evolve with population time.

## SIMULATION OF 2D SPECTRA

To simulate the P3HT response, we considered only transitions from the ground state to the 0–0 and 0–1 absorption peaks, since other vibronic transition are out of the excitation bandwith. The peak positions and relative weight have been extracted from linear absorption measurement by fitting a modified Franck-Condon progression, also used to extract the free exciton bandwith in the main text [4]. The analytical expressions for the different Feynman pathways can be found in Ref [1], to which we added a phenomenological dephasing rate $\gamma$ during the coherence times $t_{21}$ and $t_{43}$. Inhomogeneous broadening has been included by taking the ensemble average of 5000 energy configurations, using a normal distribution of transition frequencies with a full-width-at-half-maximum $\sigma$. We considered that the fluctuations of the 0–0 and 0–1 are fully correlated, meaning that their energy difference is kept at 180 meV and the inhomogeneous broadening only affects their relative energy with respect to the ground state. This relatively crude approximation tends to overestimate slightly the cross-peak strength, but allows us to restrain the model to a limited set of parameters. Finally, the experimental laser spectrum has been used to correct the calculated nonlinear responses, and to facilitate visual comparison with the experimental data. As shown in Fig. S5, since the first two peaks of the vibronic progression are broader than the laser bandwidth, the laser spectrum affects strongly the 2D spectral shape and cannot be neglected.

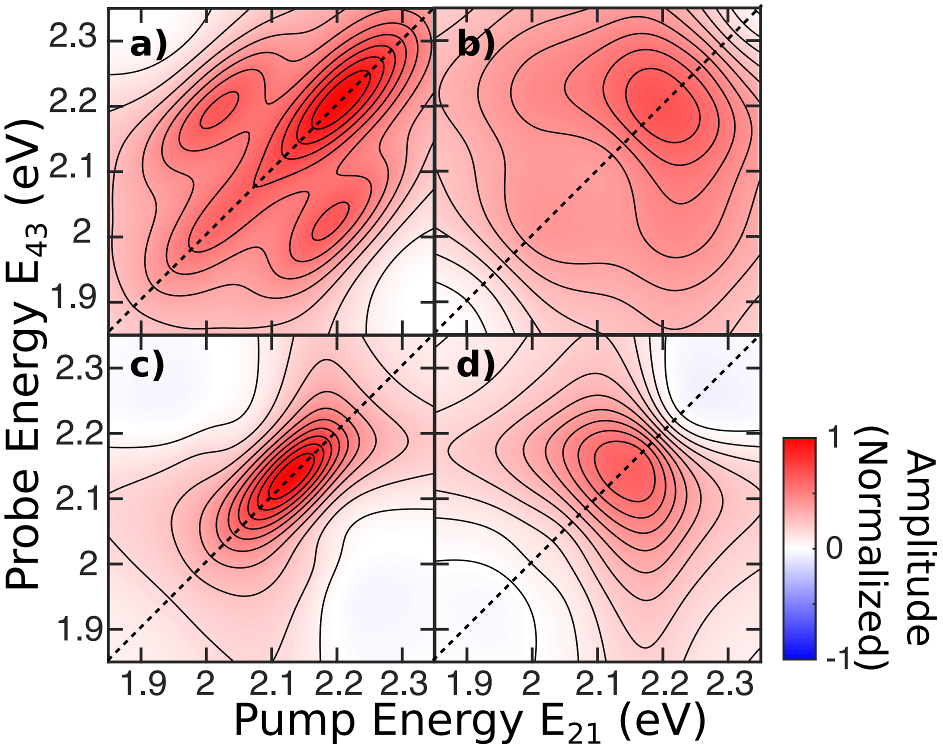


FIG. S5. Effect of the limited laser bandwidth on the simulated spectra. (a) and (b) display the real part of the rephasing and nonrephasing spectra, respectively, without taking the laser spectrum into account. (c) and (d) show the same spectra corrected for the experimental laser response.

## EXCITON ENERGY FLUCTUATIONS AND $T_2$ TIMES.

We consider a simple 2D model of a series of stacked linear polymer chains where $t$ is the intra-chain hopping integral, $J$ is the inter-chain hopping integral, and we have a total of $L_x$ monomer units along each polymer chain and $L_y$ stacked chains. The free-exciton model gives the energy as

$$E(k_x, k_y) = E_o + 2t\cos\left[\frac{\pi}{L_x+1}k_x\right] + 2J\cos\left[\frac{\pi}{L_y+1}k_y\right] \tag{1}$$

where we introduce $k_x$ and $k_y$ as quantum numbers and $E_o$ the exciton energy of a single monomer unit. Expanding this in terms of $k_x$ and $k_y$

$$E(k_x, k_y) = E_o - 2t\left[\frac{\pi}{L_x+1}\right]^2 k_x^2 - 2J\left[\frac{\pi}{L_y+1}\right]^2 k_y^2 + \cdots . \tag{2}$$

Since we are interested in the energy fluctuations, let's write $E = \overline{E} + \delta E$ by introducing the mappings $k_x \to \overline{k}_x + \delta k_x$ and $k_y \to \overline{k}_y + \delta k_y$

$$E(k_x, k_y) = \overline{E}(\overline{k}_x, \overline{k}_y) - 4\left\{t\left[\frac{\pi}{L_x+1}\right]^2 \overline{k}_x \delta k_x + J\left[\frac{\pi}{L_y+1}\right]^2 \overline{k}_y \delta k_y\right\} + \cdots . \tag{3}$$

for the lowest lying excitons, $\overline{k}_x = \overline{k}_y = 1$ and taking $L_x \gg 1$

$$\delta E_{11} = -4\left\{t\left[\frac{\pi}{L_x}\right]^2 \delta k_x + J\left[\frac{\pi}{L_y+1}\right]^2 \delta k_y\right\} + \cdots . \tag{4}$$

The dephasing time is given by $T_2 = \hbar/\sqrt{\overline{\delta E_{11}^2}}$. If we ignore the $\pi$-stacking and only have a single, isolated chain, then

$$T_{2,iso} \propto \frac{\hbar}{t\pi^2} L_x^2 \tag{5}$$

On the other hand, if we are in the aggregate domain where polymer chains are $\pi$-stacked but with the intermolecular length still greater than the intra-molecular length, i.e. $L_x \gg L_y$.

$$\sqrt{\overline{\delta E_{11}^2}} = -4\pi^2\left\{\frac{J}{(L_y+1)^2}\left[1 + \frac{t}{J}\left(\frac{L_y+1}{L_x}\right)^2\right]\right\} \tag{6}$$

implying that

$$T_{2,agg} \propto \frac{\hbar}{\pi^2 J}(L_y+1)^2\left[1 - \frac{t}{J}\left(\frac{(L_y+1)}{L_x}\right)^2 + \cdots\right] \tag{7}$$

The ratio $T_{2,agg}/T_{2,iso}$ gives the relation given in the text.

---

* e-mail: carlos.silva@umontreal.ca

[1] P. F. Tekavec, G. a. Lott, and A. H. Marcus, The Journal of Chemical Physics **127**, 214307 (2007).

[2] A. Tokmakoff, The Journal of Physical Chemistry A **104**, 4247 (2000).

[3] P. Hamm and M. Zanni, *Concepts and Methods of 2D Infrared Spectroscopy* (Cambridge University Press, 2011) p. 286.

[4] J. Clark, C. Silva, R. Friend, and F. Spano, Physical Review Letters **98**, 206406 (2007).
